# Supplementary material for: EnsIR: An Ensemble Algorithm for Image Restoration via Gaussian Mixture Models
Source: arXiv:2410.22959 source file (2024-10-30)
Supplement: Supplementary file 1 [file 7_supple_.tex]

\newpage
\appendix

\section*{Appendix}

\section{Proof}

\setcounter{theorem}{0}

\subsection{Proof of Theorem~\ref{theorem_bonferroni}}
\begin{proof}

\begin{theorem}\label{theorem_bonferroni}
    (Bonferroni's Inequality)
    Suppose \(X_1,..., X_n\) are \(n\) events. 
    Then we have the event \(X = \bigcap\limits_{i=1}^n X_i\) such that the probability distribution function \(P(X) \ge \sum\limits_{i=1}^n P(X_i) - (n-1) \) holds.
\end{theorem}
By Theorem~\ref{theorem_bonferroni}, we can find the lower bound of the likelihood of \(\mathbf{y}_{1:N}\) as 
\begin{equation}
\begin{split}
    & P(\mathbf{y}_{1:N}) \ge \sum_{r=1}^{T^M}  P(\mathbf{y}_{r,1:N}) - (T^M-1), \\
    % &\text{where } P(\mathbf{y}_{r,1:N}) = \phi\left( \mathbf{y}_{r,1:N} \left| \sum_{m=1}^M \bm{\alpha}_{r,m} \cdot \mathbf{x}_{r,m,1:N}, \sum_{m=1}^M \bm{\alpha}_{r,m}^\top \bm{\alpha}_m \cdot\mathbf{\Sigma}_{r,m,1:N}\right.\right), 
\end{split}
\end{equation}
Because there is no intersection between two bin sets, we can safely separate the optimization of maximum likelihood over \(\mathbf{y}_{1:N}\) into \(T^M\) optimization problems of maximum likelihood over \(\mathbf{y}_{r,1:N}\).

We prove Bonferroni's Inequality by induction.
We first consider the case of \(n=1\), and it holds
\begin{equation}
    P(X) = P(X_1) - (1-1)= P(X_1).
\end{equation}
When \(n=2\), we first consider the De Morgan's Law,
\begin{equation}
    \left(\bigcap\limits_{i=1}^{k} X_i\right)^c = \bigcup\limits_{i=1}^{k} X_i^c,
\end{equation}
where the super-script \((\cdot)^c\) denotes the complement of an event.
We also have Boole's Inequality.
\begin{theorem}\label{theorem_boole}
    (Boole's Inequality)
    Suppose \(X_1,..., X_n\) are \(n\) events. 
    Then we have the event \(X = \bigcup_{i=1}^n X_i\) such that the probability distribution function \(P(X) \le \sum_i^n P(X_i) \) holds.
\end{theorem}
Based on the two properties above, we have Bonferroni's Inequality holds when \(n=2\):
\begin{equation}
\begin{split}
    P(X_1 \cap X_2) &= 1 - P\left((X_1 \cap X_2 )^c\right) \\
    & = 1 - P(X_1^c \cup X_2^c ) \\
    & \ge 1 - \sum_{i=1}^2 P(X_1^c) \\ 
    & = \sum_{i=1}^2 P(X_i) - 1 .
\end{split}
\end{equation}

When \(n = k\), suppose we have the following inequality holds
\begin{equation}
    P\left(\bigcap\limits_{i=1}^k X_i\right) \ge \sum_{i=1}^k P(X_i) - (k-1).
\end{equation}

We now want to prove the inequality for the case of \(n=k+1\),
\begin{equation}
\begin{split}
    P\left(\bigcap_{i=1}^{k+1} X_i \right) &= P\left( \left(\bigcap_{i=1}^{k} X_i \right) \cap X_{k+1} \right) \\
    & = P\left( \bigcap_{i=1}^{k} X_i \right) + P(X_{k+1}) - P\left( \left(\bigcap_{i=1}^{k} X_i \right) \cup X_{k+1} \right) \\ 
    & \ge \sum_{i=1}^k P(X_i) - (k-1) + P(X_{k+1}) - P\left( \left(\bigcap_{i=1}^{k} X_i \right) \cup X_{k+1} \right) \\
    & = \sum_{i=1}^{k+1} P(X_i) - (k-1)- P\left( \left(\bigcap_{i=1}^{k} X_i \right) \cup X_{k+1} \right) \\
    & \ge \sum_{i=1}^{k+1} P(X_i) - (k+1-1) \\
\end{split}
\end{equation}
Therefore, we complete the proof.
\end{proof}

\subsection{Convergence of GMMs with prior means}

\subsection{Proof of Theorem~\ref{theorem2}}

Maximum likelihood estimation
\begin{equation}
\begin{split}
    f_1 &= \mathop{\arg\max}\limits_{f_1} \{\log P(\mathbf{Y}_n | f_1, \mathbf{X}_n)\} = \mathop{\arg\max}\limits_{f_1} \sum_{n=1}^N \log   \mathcal{N}(\mathbf{Y}_n | f_1(\mathbf{X}_n),\mathbf{\Sigma}_{1,n}) \\
    &= \mathop{\arg\min}\limits_{f_1} \sum_{n=1}^N \|f_1(\mathbf{X}_n) - \mathbf{Y}_n\|_2^2  
\end{split}
\end{equation}
\subsection{Proof of Decreasing Variance of Ensemble}

\section{Preparing PDF files}

Please prepare submission files with paper size ``US Letter,'' and not, for
example, ``A4.''

Fonts were the main cause of problems in the past years. Your PDF file must only
contain Type 1 or Embedded TrueType fonts. Here are a few instructions to
achieve this.

\begin{itemize}

\item You should directly generate PDF files using \verb+pdflatex+.

\item You can check which fonts a PDF files uses.  In Acrobat Reader, select the
  menu Files$>$Document Properties$>$Fonts and select Show All Fonts. You can
  also use the program \verb+pdffonts+ which comes with \verb+xpdf+ and is
  available out-of-the-box on most Linux machines.

\item \verb+xfig+ "patterned" shapes are implemented with bitmap fonts.  Use
  "solid" shapes instead.

\item The \verb+\bbold+ package almost always uses bitmap fonts.  You should use
  the equivalent AMS Fonts:
\begin{verbatim}
   \usepackage{amsfonts}
\end{verbatim}
followed by, e.g., \verb+\mathbb{R}+, \verb+\mathbb{N}+, or \verb+\mathbb{C}+
for $\mathbb{R}$, $\mathbb{N}$ or $\mathbb{C}$.  You can also use the following
workaround for reals, natural and complex:
\begin{verbatim}
   \newcommand{\RR}{I\!\!R} %real numbers
   \newcommand{\Nat}{I\!\!N} %natural numbers
   \newcommand{\CC}{I\!\!\!\!C} %complex numbers
\end{verbatim}
Note that \verb+amsfonts+ is automatically loaded by the \verb+amssymb+ package.

\end{itemize}

If your file contains type 3 fonts or non embedded TrueType fonts, we will ask
you to fix it.

\subsection{Margins in \LaTeX{}}

Most of the margin problems come from figures positioned by hand using
\verb+\special+ or other commands. We suggest using the command
\verb+\includegraphics+ from the \verb+graphicx+ package. Always specify the
figure width as a multiple of the line width as in the example below:
\begin{verbatim}
   \usepackage[pdftex]{graphicx} ...
   \includegraphics[width=0.8\linewidth]{myfile.pdf}
\end{verbatim}
See Section 4.4 in the graphics bundle documentation
(\url{http://mirrors.ctan.org/macros/latex/required/graphics/grfguide.pdf})

A number of width problems arise when \LaTeX{} cannot properly hyphenate a
line. Please give LaTeX hyphenation hints using the \verb+\-+ command when
necessary.

\begin{ack}
Use unnumbered first level headings for the acknowledgments. All acknowledgments
go at the end of the paper before the list of references. Moreover, you are required to declare
funding (financial activities supporting the submitted work) and competing interests (related financial activities outside the submitted work).
More information about this disclosure can be found at: \url{https://neurips.cc/Conferences/2024/PaperInformation/FundingDisclosure}.

Do {\bf not} include this section in the anonymized submission, only in the final paper. You can use the \texttt{ack} environment provided in the style file to automatically hide this section in the anonymized submission.
\end{ack}

\section*{References}

References follow the acknowledgments in the camera-ready paper. Use unnumbered first-level heading for
the references. Any choice of citation style is acceptable as long as you are
consistent. It is permissible to reduce the font size to \verb+small+ (9 point)
when listing the references.
Note that the Reference section does not count towards the page limit.
